# Supplementary material for: Rhetoric, Logic, and Dialectic: Advancing Theory-based Argument Quality Assessment in Natural Language Processing
Source: arXiv:2006.00843 source file (2020-11-03)
Supplement: Supplementary file 1 [file appendix.tex]

\section*{Details about Crowd-sourcing Studies}
\subsection*{Selecting Argumentative CQA Posts}
When sampling posts from Yahoo! Answers for the CQA domain, our goal was to have a high proportion of argumentative texts. Therefore, we conducted a secondary experiment on Amazon Mechanical Turk to select posts likely to be argumentative.  
Participants had to meet the following qualifications: HIT approval rate $\geq$ $97$; HITs approved $>$ $500$; Location = US.
We randomly selected 5,000 posts from the \emph{Politics \& Government $\rightarrow$ Law \& Ethics} subcategory that were labeled to be the best answer. For each post, we collected $10$ binary judgments about whether the text contained an argument. 
In our annotation study, we only include posts that a majority of raters labeled \textit{argumentative} (this threshold was selected by manual inspection).  %\jttodo{do we have statistics on how well Turkers fared at this task?  Someone is going to ask this...}\altodo{I have Krippendorff for all MTurk tasks -LN} 

\subsection*{Annotation Details}
%\altodo{what is QA here?}
All of the contributors we worked with on Appen were native English speakers, % paid \$0.45--\$0.65 per judgment (increased over time). \todocn{I removed this part since we don't have the same information for turk we need to add ths to the final paper}
and we manually reviewed the judgments in pilot studies to remove underperforming annotators. We measured inter-annotator agreements with Krippendorff's alpha and MACE \cite{hovy-etal-2013-learning}. Krippendorff's alpha per annotator was calculated by comparing each annotator's judgments to the rest of the group's for each dimension and averaging the results. Annotators who had an average Krippendorff's alpha lower than $0.1$ were blocked from participating in further rounds.

\section*{Extended Model Descriptions}
Here, we provide extended descriptions for the models employed in our experiments.

We employ the scikit-learn toolkit %\cntodo{fill in}
for the SVR models. The \textsc{BERT}-based models rely on a pretrained multi-layer bidirectional Transformer \cite{vaswani2017attention}. To this end, we transform each argument into a ``BERT-compatible'' format, i.e., into a sequence of WordPiece \cite{wu2016google} tokens and prepend the whole sequence with \textsc{BERT}'s sequence start token (\texttt{[CLS]}). The pooled hidden representation of the latter corresponds to the aggregated document representation $\textbf{h}_\mathit{D} \in \mathbb{R}^h$.
%We experiment with the plain pretrained BERT variants, BERT$_{Base}$ and BERT$_{Large}$, as well as with BERT on STILTS \cite{phang_stilts}.
% We describe the score prediction layers,  and training objectives employed in our  single-task and multi-task learning experiments.
The specific details of each model are described below.
% %Given the need for a more fine-grained prediction of AQ scores combined with the availability of \corpus, 
% we next describe one correlation-based baseline, three Support Vector Regression (SVR) based models %\jttodo{it's actually three SVRs and one length one right?} 
% and three BERT-based \cite{devlin2018bert} AQ prediction architectures, which we employ to further answer \textbf{RQ2}--\textbf{RQ4}: 

% For addressing the question whether we are able to develop a computational theory-based AQ model (\textbf{RQ2}), we employ: (1) \textsc{Arg Length}, (2) \textsc{SVR$_{tfidf}$}, (3) \textsc{SVR$_{embd}$}, %(4) \textsc{Wachsmuth$_{All}$}, 
% (4) \textsc{Wachsmuth$_{CFS}$}, and (5) \textsc{BERT ST}. 

\paragraph{Argument Length (\textsc{Arg length}).} To estimate the task difficulty and to measure a potential length bias, our naive baseline is the correlation between the argument's character length and quality scores.%\cntodo{test score? should be quality score?}\jttodo{why characters instead of words?}

\paragraph{SVR with Lexical Features (\textsc{SVR$_{tfidf}$}).} We run a simple SVR with tf--idf feature vectors. %\jttodo{which toolkit}

\paragraph{SVR with Semantic Features (\textsc{SVR$_{embd}$}).} We represent each argument as the average of the fastText~\cite{Bojanowski:2017tacl} embedding\footnote{\url{https://dl.fbaipublicfiles.com/fasttext/vectors-english/wiki-news-300d-1M-subword.vec.zip}} representation of each word in the argument.

\paragraph{Feature-rich SVR (\textsc{Wachsmuth$_{CFS}$}).}
%(\textsc{Wachsmuth$_{All}$}).}: Further, we replicate the approach of \newcite{wachsmuth-etal-2016-using}, who employ a rich set of features including standard features (e.g., token n-grams, part-of-speech tags, etc.) as well as higher-level features (e.g., sentiment flows, argumentative discourse units etc.), which they then use as input for an SVR. For this variant of the approach, we employ all features.
%
%\vspace{0.4em}
%\noindent 
 We reimplement %\jttodo{can we say reimplement? We mostly used hennings code} 
 the approach of \newcite{wachsmuth-etal-2016-using}, who employ standard features (token n-grams, part-of-speech tags, etc.) and higher-level features (sentiment flows, argumentative discourse units etc.). We run correlation-based feature selection on the training set and include only the most predictive features.

% \noindent The \textsc{BERT}-based models rely on a pretrained multi-layer bidirectional Transformer \cite{vaswani2017attention}. To this end, we transform each argument into a ``BERT-compatible'' format, i.e., into a sequence of WordPiece \cite{wu2016google} tokens and prepend the whole sequence with \textsc{BERT}'s sequence start token (\texttt{[CLS]}). The pooled hidden representation of the latter corresponds to the aggregated document representation $h_D \in \mathbb{R}^h$.
%We experiment with the plain pretrained BERT variants, BERT$_{Base}$ and BERT$_{Large}$, as well as with BERT on STILTS \cite{phang_stilts}.
%We describe the score prediction layers,  and training objectives employed in our  single-task and multi-task learning experiments.
\paragraph{Single Task Learning Setting (\textsc{BERT ST}).} For each AQ dimension $t$, we train an individual regressor.  Let $\textbf{h}_\mathit{D} \in \mathbb{R}^h$ be the vector representation of the argument. %\footnote{For the recurrent encoders, $\textbf{h}_\mathit{D}$ corresponds to the aggregation of the contextualized sentence or token representations, while for BERT-based models $\textbf{h}_\mathit{D} \in \mathbb{R}^h$ is the transformed vector representation of the sequence start token [CLS] that encodes the whole sequence.}   
  Our AQ predictor is a simple linear regression layer with $\mathbf{W}_{\mathit{t}} \in \mathbb{R}^{H}$ and $\mathbf{b}_{\mathit{t}} \in \mathbb{R}$ as the classifier's trainable parameters:
$
    \hat{\mathbf{y}} = \mathbf{h}_{\mathit{D}}\mathbf{W}_{\mathit{t}}^\top + \mathbf{b}_{\mathit{t}}\,.
    \label{eq:PredictionT}
$
The loss $L_{\mathit{t}}$ is then simply the mean squared error (MSE) over $k$ instances in the training batch, where $\mathbf{y} \in [0;5]$ is the true score for a training instance for the dimension $t$:
$
    L_{\mathit{t}} = \frac{1}{k}\sum^{k}_{i=0}(y_i-\hat{y}_i)^2.
    \label{eq:LossT}
$
\paragraph{Flat Multi-Task Learning Setting (\textsc{BERT MT$_{flat}$}).} %Each individual argument has four quality scores
%reflecting cogency, effectiveness, reasonableness, and overall quality, which are related, as shown by correlation analysis \cite{wachsmuth-etal-2017-computational}. 
We explore whether a joint training setup would improve the individual score predictions. Let $\textbf{h}_\mathit{D} \in \mathbb{R}^h$ be the vector representation of the argument. For each quality dimension, we employ an individual prediction layer and compute an individual task loss $L_{\mathit{t}}$. We then define the total training loss $L_{Total}$ as the sum of the task losses $L_{\mathit{t}}$, with $T=\{\textnormal{Cogency}, \textnormal{Effectiveness}, \textnormal{Reasonableness}, \textnormal{Overall Quality}\}$ as the set of AQ  dimensions:
$
    L_{\mathit{Total}} = \sum_{t \in T} L_{\mathit{t}}\,.
    \label{eq:LossFlat}
$

\paragraph{Hierarchical Multi-Task Learning Setting (\textsc{BERT MT$_{hier}$}).} %The taxonomy presented by \newcite{wachsmuth-etal-2017-computational} exhibits an hierarchical relationship between the three sub-dimensions cogency, effectiveness, and reasonableness, versus overall argument quality. In order to study whether it is possible to exploit this hierarchical relationship (\textbf{RQ3}), 
We propose a hierarchical multi-task learning setting to exploit the hierarchical relationship between the scores. Similar to above, we first learn jointly the lower-level tasks (Cogency, Effectiveness, Reasonableness) resulting in three scores $\hat{y}_{\textnormal{Cog}}$, $\hat{y}_{\textnormal{Eff}}$ and $\hat{y}_{\textnormal{Rea}}$. Next, we employ these scores for informing the overall argument quality predictor by concatenating these with the hidden document representation $\textbf{h}_\mathit{D}$:
$
    \mathbf{h}_{\mathit{informed}} = \mathbf{h}_{D}^\frown [\hat{y}_{\textnormal{Cog}}, \hat{y}_{\textnormal{Eff}},\hat{y}_{\textnormal{Rea}}].
    %\label{eq:LossT}
$
The resulting vector $h_{\mathit{informed}}$ serves as input to the overall AQ predictor as defined in before. 

\section*{Experimental Details}
\subsection*{Hyperparameter Optimization}
\begin{table}[!th]\centering
\small
\begin{tabular}{llr}\toprule
Model Type & Hyperparameter &Values \\\midrule
\multirow{2}{*}{SVR} &Regularization $c$ &$0.001$, $0.01$, $0.1$, $1.0$, $10$ \\
&Epsilon-tube specifier $\epsilon$ &$0.001$, $0.01$, $0.1$, $1.0$ \\
\multirow{2}{*}{BERT} &Learning rate $\lambda$ &$2 \cdot 10^{-5}$, $3 \cdot 10^{-5}$ \\
&Number of Epochs &$3$,$4$ \\
\bottomrule
\end{tabular}
\caption{Search values per model type and hyperparameter employed in the experiments for answering RQ2--RQ5. }\label{tab:hyper}
\end{table}
For each experiment, we conducted a grid search on the corresponding development portion of the employed training set. The search spaces are depicted in Table~\ref{tab:hyper}.

\subsection*{Full Experimental Results for RQ2--RQ4}
In the following, we list the full experimental results on \corpus with respect to the research questions RQ2--RQ4.

\setlength{\tabcolsep}{4pt}
\begin{table*}[th]\centering
\small
\begin{tabular}{llrrrrrrrrrr}\toprule
 &\textbf{} &\multicolumn{3}{c}{\textbf{CQA forums}} &\multicolumn{3}{c}{\hspace{1em}\textbf{Debate Forums}} &\multicolumn{3}{c}{\hspace{1em}\textbf{Review Forums}} \\\cmidrule{3-11}
&\textbf{Model} &\textbf{Crowd} &\textbf{Expert} &\textbf{Mix} &\hspace{1em}\textbf{Crowd} &\textbf{Expert} &\textbf{Mix} &\hspace{1em}\textbf{Crowd} &\textbf{Expert} &\textbf{Mix} \\\midrule
\multirow{5}{*}{\textbf{Overall}} &\textsc{Arg length} &0.498 &0.236 &0.406 &0.542 &0.232 &0.420 &0.486 &0.190 &0.365 \\
%&\textsc{Wachsmuth$_{\textit{All}$}} &0.331 &0.224 &0.307 &0.341 &0.176 &0.284 &0.481 &0.188 &0.360 \\
&\textsc{SVR$_{\textit{tfidf}}$} &0.381 &0.323 &0.389 &0.299 &0.179 &0.265 &0.446 &0.340 &0.450 \\
&\textsc{SVR$_{\textit{embd}}$} &0.323 &0.180 &0.278 &0.467 &0.239 &0.388 &0.223 &0.227 &0.265 \\
&\textsc{Wachsmuth$_{\textit{CFS}}$} &0.550 &0.340 &0.492 &0.524 &0.264 &0.432 &\textbf{0.619} &0.342 &0.533 \\
&\textsc{BERT ST} &\textbf{0.681} & \textbf{0.498} & \textbf{0.652} & \textbf{0.575} & \textbf{0.346} & \textbf{0.511} &0.611 & \textbf{0.450} &\textbf{0.605} \\
%&\textsc{BERT MT$_{\textit{flat}$}} &0.671 &\textbf{0.535} &\textbf{0.667} &\textbf{0.607} &\textbf{0.362} &\textbf{0.537} &0.534 &\textbf{0.478} &0.588 \\
%&\textbf{\textsc{BERT MT$_{\textit{hier}$}}}  &0.668 &0.528 &0.661 &0.480 &0.393 &0.494 &0.563 &0.465 &0.593 \\
\midrule
\multirow{5}{*}{\textbf{Cogency}} & \textsc{Arg length} &0.502 &0.227 &0.420 & \textbf{0.574} &0.225 &0.437 &0.491 &0.125 &0.340 \\ %&\textsc{Wachsmuth$_{\textit{All}$}}  &0.291 &0.161 &0.259 &0.278 &0.120 &0.219 &0.493 &0.043 &0.287 \\
&\textsc{SVR$_{\textit{tfidf}}$} &0.449 &0.330 &0.444 &0.295 &0.164 &0.257 &0.409 &0.264 &0.384 \\
&\textsc{SVR$_{\textit{embd}}$} &0.301 &0.154 &0.261 &0.404 &0.196 &0.333 &0.264 &-0.059 &0.103 \\
&\textsc{Wachsmuth$_{\textit{CFS}}$} &0.565 &0.311 &0.503 &0.548 &0.232 &0.429 &0.611 &0.223 &0.464 \\
&\textsc{BERT ST} & \textbf{0.623} & \textbf{0.405} & \textbf{0.587} & 0.556 & \textbf{0.337} & \textbf{0.503} &\textbf{0.618} & \textbf{0.359} & \textbf{0.554} \\
%&\textsc{BERT MT$_{\textit{flat}$}} &\textbf{0.651} &0.457 &0.633 &\textbf{0.622} &0.343 &\textbf{0.541} &0.533 &\textbf{0.440} &\textbf{0.561} \\
%&\textbf{\textsc{BERT MT$_{\textit{hier}$}}}  &0.650 &\textbf{0.468} &\textbf{0.638} &0.476 &\textbf{0.353} &0.474 &0.559 &0.388 &0.541 \\
\midrule
\multirow{5}{*}{\textbf{Effectiveness}} & \textsc{Arg length} &0.475 &0.237 &0.390 &0.502 &0.225 &0.399 &0.425 &0.251 &0.372 \\ %&\textsc{Wachsmuth$_{\textit{All}$}}  &0.333 &0.203 &0.295 &0.274 &0.194 &0.265 &0.471 &0.171 &0.336 \\
&\textsc{SVR$_{\textit{tfidf}}$} &0.432 &0.313 &0.411 &0.141 &0.074 &0.120 &0.354 &0.253 &0.340 \\
&\textsc{SVR$_{\textit{embd}}$} &0.328 &0.204 &0.293 &0.456 &0.264 &0.403 &0.186 &0.144 &0.187 \\
&\textsc{Wachsmuth$_{\textit{CFS}}$} &0.555 &0.393 &0.523 &0.528 &0.281 &0.450 &0.567 &0.246 &0.432 \\
&\textsc{BERT ST} & \textbf{0.596} & \textbf{0.509} & \textbf{0.612} & \textbf{0.548} & \textbf{0.405} & \textbf{0.542} &\textbf{0.639} & \textbf{0.370} &\textbf{0.555} \\
%&\textsc{BERT MT$_{\textit{flat}$}} &\textbf{0.663} &0.549 &\textbf{0.671} &\textbf{0.599} &0.408 &\textbf{0.570} &0.522 &\textbf{0.389} &0.514 \\
%&\textbf{\textsc{BERT MT$_{\textit{hier}$}}}  &0.656 &\textbf{0.552} &0.670 &0.477 &\textbf{0.443} &0.532 &0.466 &0.388 &0.486 \\
\midrule
\multirow{5}{*}{\textbf{Reasonableness}} & \textsc{Arg length} &0.480 &0.245 &0.396 &0.535 &0.170 &0.377 &0.496 &0.241 &0.405 \\ %&\textsc{Wachsmuth$_{\textit{All}$}}  &0.313 &0.215 &0.290 &0.320 &0.097 &0.223 &0.453 &0.169 &0.332 \\
&\textsc{SVR$_{\textit{tfidf}}$} &0.466 &0.364 &0.457 &0.292 &0.153 &0.247 &0.435 &0.345 &0.452 \\
&\textsc{SVR$_{\textit{embd}}$}&0.411 &0.278 &0.379 &0.393 &0.096 &0.258 &0.205 &0.191 &0.234 \\
&\textsc{Wachsmuth$_{\textit{CFS}}$} &0.543 &0.326 &0.476 &\textbf{.549} &0.192 &0.399 &0.524 &0.261 &0.432 \\
&\textsc{BERT ST} &\textbf{0.696} &\textbf{0.512} &\textbf{0.665} & 0.544 & \textbf{0.222} & \textbf{0.418} &\textbf{0.556} & \textbf{0.484} & \textbf{0.609} \\
%&\textsc{BERT MT$_{\textit{flat}$}} &0.672 &0.499 &0.644 &\textbf{0.587} &0.273 &\textbf{0.473} &0.550 &\textbf{0.489} &0.610 \\
%&\textbf{\textsc{BERT MT$_{\textit{hier}$}}}  &0.660 &0.478 &0.626 &0.445 &\textbf{0.280} &0.408 &0.555 &0.488 &\textbf{0.611} \\
\bottomrule
\end{tabular}
\caption{Pearson correlations of our model predictions with the annotation scores for the four AQ dimensions on the three different test annotations (Crowd, Expert, Mix) when training on in-domain data. Numbers in bold indicate best performances.
}
\end{table*}
\setlength{\tabcolsep}{4pt}
\begin{table*}[th]\centering
\small
\begin{tabular}{llrrrrrrrrrr}\toprule
 &\textbf{} &\multicolumn{3}{c}{\hspace{1em}\textbf{CQA forums}} &\multicolumn{3}{c}{\hspace{1em}\textbf{Debate Forums}} &\multicolumn{3}{c}{\hspace{1em}\textbf{Review Forums}} \\\cmidrule{3-11}
&\textbf{Model} &\hspace{1em}\textbf{Crowd} &\textbf{Expert} &\textbf{Mix} &\hspace{1em}\textbf{Crowd} &\textbf{Expert} &\textbf{Mix} &\hspace{1em}\textbf{Crowd} &\textbf{Expert} &\textbf{Mix} \\\midrule
\multirow{3}{*}{\textbf{Overall}} %&\textsc{Arg length} &0.498 &0.236 &0.406 &0.542 &0.232 &0.420 &0.486 &0.190 &0.365 \\
%&\textsc{Wachsmuth$_{\textit{All}$}} &0.331 &0.224 &0.307 &0.341 &0.176 &0.284 &0.481 &0.188 &0.360 \\
%&\textsc{Wachsmuth$_{\textit{CFS}$}} &0.550 &0.340 &0.492 &0.524 &0.264 &0.432 &\textbf{0.619} &0.342 &0.533 \\
%&%}$}} &0.381 &0.323 &0.389 &0.299 &0.179 &0.265 &0.446 &0.340 &0.450 \\
%&\textsc{SVR$_{\textit{embd}$}} &0.323 &0.180 &0.278 &0.467 &0.239 &0.388 &0.223 &0.227 &0.265 \\
&\textsc{BERT ST} &\textbf{0.681} &0.498 &0.652 &0.575 &0.346 &0.511 & \textbf{0.611} &0.450 &\textbf{0.605} \\
&\textsc{BERT MT$_{\textit{flat}}$} &0.671 &\textbf{0.535} &\textbf{0.667} &\textbf{0.607} &\textbf{0.362} &\textbf{0.537} &0.534 &\textbf{0.478} &0.588 \\
&\textsc{BERT MT$_{\textit{hier}}$}  &0.668 &0.528 &0.661 &0.480 &0.393 &0.494 &0.563 &0.465 &0.593 \\
\midrule
\multirow{3}{*}{\textbf{Cogency}} %& \textsc{Arg length} &0.502 &0.227 &0.420 &0.574 &0.225 &0.437 &0.491 &0.125 &0.340 \\ &\textsc{Wachsmuth$_{\textit{All}$}}  &0.291 &0.161 &0.259 &0.278 &0.120 &0.219 &0.493 &0.043 &0.287 \\
%&\textsc{Wachsmuth$_{\textit{CFS}$}} &0.565 &0.311 &0.503 &0.548 &0.232 &0.429 &0.611 &0.223 &0.464 \\
%&\textsc{SVR$_{\textit{tfidf}$}} &0.449 &0.330 &0.444 &0.295 &0.164 &0.257 &0.409 &0.264 &0.384 \\
%&\textsc{SVR$_{\textit{embd}$}} &0.301 &0.154 &0.261 &0.404 &0.196 &0.333 &0.264 &-0.059 &0.103 \\
&\textsc{BERT ST} &0.623 &0.405 &0.587 &0.556 &0.337 &0.503 &\textbf{0.618} &0.359 &0.554 \\
&\textsc{BERT MT$_{\textit{flat}}$} &\textbf{0.651} &0.457 &0.633 &\textbf{0.622} &0.343 &\textbf{0.541} &0.533 &\textbf{0.440} &\textbf{0.561} \\
&\textsc{BERT MT$_{\textit{hier}}$}  &0.650 &\textbf{0.468} &\textbf{0.638} &0.476 &\textbf{0.353} &0.474 &0.559 &0.388 &0.541 \\
\midrule
\multirow{3}{*}{\textbf{Effectiveness}} %& \textsc{Arg length} &0.475 &0.237 &0.390 &0.502 &0.225 &0.399 &0.425 &0.251 &0.372 \\ &\textsc{Wachsmuth$_{\textit{All}$}}  &0.333 &0.203 &0.295 &0.274 &0.194 &0.265 &0.471 &0.171 &0.336 \\
%&\textsc{Wachsmuth$_{\textit{CFS}$}} &0.555 &0.393 &0.523 &0.528 &0.281 &0.450 &0.567 &0.246 &0.432 \\
%&\textsc{SVR$_{\textit{tfidf}$}} &0.432 &0.313 &0.411 &0.141 &0.074 &0.120 &0.354 &0.253 &0.340 \\
%&\textsc{SVR$_{\textit{embd}$}} &0.328 &0.204 &0.293 &0.456 &0.264 &0.403 &0.186 &0.144 &0.187 \\
&\textsc{BERT ST} &0.596 &0.509 &0.612 &0.548 &0.405 &0.542 &\textbf{0.639} &0.370 &\textbf{0.555} \\
&\textsc{BERT MT$_{\textit{flat}}$} &\textbf{0.663} &0.549 &\textbf{0.671} &\textbf{0.599} &0.408 &\textbf{0.570} &0.522 &\textbf{0.389} &0.514 \\
&\textsc{BERT MT$_{\textit{hier}}$}  &0.656 &\textbf{0.552} &0.670 &0.477 &\textbf{0.443} &0.532 &0.466 &0.388 &0.486 \\
\midrule
\multirow{3}{*}{\textbf{Reasonableness}} %& \textsc{Arg length} &0.480 &0.245 &0.396 &0.535 &0.170 &0.377 &0.496 &0.241 &0.405 \\ &\textsc{Wachsmuth$_{\textit{All}$}}  &0.313 &0.215 &0.290 &0.320 &0.097 &0.223 &0.453 &0.169 &0.332 \\
%&\textsc{Wachsmuth$_{\textit{CFS}$}} &0.543 &0.326 &0.476 &0.549 &0.192 &0.399 &0.524 &0.261 &0.432 \\
%&\textsc{SVR$_{\textit{tfidf}$}} &0.466 &0.364 &0.457 &0.292 &0.153 &0.247 &0.435 &0.345 &0.452 \\
%&\textsc{SVR$_{\textit{embd}$}}&0.411 &0.278 &0.379 &0.393 &0.096 &0.258 &0.205 &0.191 &0.234 \\
&\textsc{BERT ST} &\textbf{0.696} &\textbf{0.512} &\textbf{0.665} &0.544 &0.222 &0.418 &\textbf{0.556} &0.484 &0.609 \\
&\textsc{BERT MT$_{\textit{flat}}$} &0.672 &0.499 &0.644 &\textbf{0.587} &0.273 &\textbf{0.473} &0.550 &\textbf{0.489} &0.610 \\
&\textsc{BERT MT$_{\textit{hier}}$}  &0.660 &0.478 &0.626 &0.445 &\textbf{0.280} &0.408 &0.555 &0.488 &\textbf{0.611} \\
\bottomrule
\end{tabular}
\caption{Pearson correlations of our model predictions with the annotation scores. %for the four argument quality dimensions on the three different test annotations for three domains when training on the domain-specific data only. 
 We compare single-task versus multi-task learning setups training on in-domain data only. %Numbers in bold indicate best performances.
}
\end{table*}
\setlength{\tabcolsep}{4pt}
\begin{table*}[!th]\centering
%\scriptsize
\small
\begin{tabular}{llrrrrrrrrrr}\toprule
&\textbf{} &\multicolumn{3}{c}{\hspace{1em}\textbf{CQA forums}} &\multicolumn{3}{c}{\hspace{1em}\textbf{Debate Forums}} &\multicolumn{3}{c}{\hspace{1em}\textbf{Review Forums}} \\\cmidrule{3-11}
&\textbf{Model} &\hspace{1em}\textbf{Crowd} &\textbf{Expert} &\textbf{Mix} &\hspace{1em}\textbf{Crowd} &\textbf{Expert} &\textbf{Mix} &\hspace{1em}\textbf{Crowd} &\textbf{Expert} &\textbf{Mix} \\\midrule
\multirow{6}{*}{\textbf{Overall}} &Best in-domain &0.681 &\textbf{0.535} &0.667 &\textbf{0.607} &0.362 &0.537 &0.619 & \textbf{0.478} &0.605 \\
%&\textsc{SVR$_{\textit{tfidf}$}} &0.407 &0.280 &0.379 &0.202 &0.109 &0.171 &0.570 &0.384 &0.540 \\
%&\textsc{SVR$_{\textit{embd}$}} &0.382 &0.244 &0.346 &0.388 &0.187 &0.314 &0.271 &0.136 &0.224 \\
&\textsc{BERT ST} &0.693 &0.530 &0.676 &0.571 &0.401 &0.545 &0.650 &0.409 &0.596 \\
&\textsc{BERT MT$_{\textit{flat}}$}  &\textbf{0.697} &\textbf{0.535} &\textbf{0.681} &0.574 &\textbf{0.425} &\textbf{0.562} &\textbf{0.678} &0.443 &\textbf{0.633} \\
&\textsc{BERT MT$_{\textit{hier}}$}  &0.680 &0.522 &0.665 &0.576 &0.424 &\textbf{0.562} &0.618 &0.469 &0.622 \\
\midrule
\multirow{6}{*}{\textbf{Cogency}} &Best in-domain &0.651 &0.468 &0.638 &\textbf{0.622} &0.353 &0.541 &\textbf{0.618} &0.440 &0.561 \\
%&\textsc{SVR$_{\textit{tfidf}$}} &0.374 &0.244 &0.353 &0.164 &0.184 &0.205 &0.532 &0.363 &0.511 \\
%&\textsc{SVR$_{\textit{embd}$}} &0.337 &0.171 &0.292 &0.323 &0.149 &0.261 &0.292 &-0.020 &0.143 \\
&\textsc{BERT ST} &0.639 &0.426 &0.608 &0.540 &0.367 &0.515 &0.601 &0.386 &0.563 \\
&\textsc{BERT MT$_{\textit{flat}}$}  &\textbf{0.673} &\textbf{0.472} & \textbf{0.653} &0.560 &0.392 &0.542 &0.610 &0.391 &0.570 \\
&\textsc{BERT MT$_{\textit{hier}}$}  &0.662 &0.455 &0.638 &0.573 &\textbf{0.397} &\textbf{0.552} &0.577 &\textbf{0.465} &\textbf{0.599} \\
\midrule
\multirow{6}{*}{\textbf{Effectiveness}} &Best in-domain &0.656 &0.552 &0.671 &\textbf{0.599} &0.443 &0.570 &0.639 &0.389 &0.555 \\
%&\textsc{SVR$_{\textit{tfidf}$}} &0.381 &0.264 &0.356 &0.258 &0.114 &0.204 &0.506 &0.293 &0.440 \\
%&\textsc{SVR$_{\textit{embd}$}} &0.346 &0.254 &0.331 &0.385 &0.199 &0.324 &0.245 &0.088 &0.175 \\
&\textsc{BERT ST} &0.664 &\textbf{0.574} &\textbf{0.686} &0.544 &\textbf{0.492} &\textbf{0.598} &\textbf{0.711} &0.387 &0.601 \\
&\textsc{BERT MT$_{\textit{flat}}$}  &\textbf{0.676} &0.536 &0.670 &0.569 &0.444 &0.578 &0.683 &\textbf{0.409} &\textbf{0.603} \\
&\textsc{BERT MT$_{\textit{hier}}$} &0.657 &0.523 &0.653 &0.573 &0.462 &0.592 &0.644 &0.396 &0.576 \\
\midrule
\multirow{6}{*}{\textbf{Reasonableness}} &Best in-domain &\textbf{0.696} &\textbf{0.512} &\textbf{0.665} &\textbf{0.587} &0.280 &0.473 &0.556 &\textbf{0.489} &0.611 \\
%&\textsc{SVR$_{\textit{tfidf}$}} &0.451 &0.345 &0.438 &0.240 &0.118 &0.198 &0.599 &0.422 &0.584 \\
%&\textsc{SVR$_{\textit{embd}$}} &0.486 &0.297 &0.430 &0.392 &0.189 &0.321 &0.283 &0.182 &0.263 \\
&\textsc{BERT ST} &0.658 &0.495 &0.635 &0.550 &0.320 &\textbf{0.487} &0.616 &0.437 &0.603 \\
&\textsc{BERT MT$_{\textit{flat}}$}  &0.691 &0.503 &0.657 &0.538 &\textbf{0.328} &0.486 &\textbf{0.667} &0.443 &0.631 \\
&\textsc{BERT MT$_{\textit{hier}}$} &0.665 &0.485 &0.633 &0.554 &0.312 &0.483 &0.642 &0.476 &\textbf{0.643} \\
\bottomrule
\end{tabular}
\caption{Pearson correlations of the model predictions with the annotation scores when training on the joint training sets of all domains. We compare with the best result of the in-domain setting.}
\end{table*}
\section*{Further Validation}
For further validation, in addition to only predicting on our own corpus, %\corpus
\texttt{AQCorpus}, we, again, employ Dagstuhl-ArgQuality-Corpus-V2 (\textsc{DS})  and predict theory-based AQ scores on \textsc{DS} instances. In order to obtain a single gold score per annotation instance and dimension from \textsc{DS}, we apply two ways of aggregating the annotations provided by the authors: (1) majority vote, and (2) mean aggregation. As the \textsc{BERT MT$_{Flat}$} models %\altodo{This is the problem here.} 
have shown to perform best on many setups of the previous experiments, we reuse them -- trained either on in-domain data or using data from all domains on \texttt{AQCorpus} -- and predict AQ dimension scores on the whole \textsc{DS} corpus. %\altodo{I need to rerun the experiments with the ST models because I employed the MT models and at this point in time, they are not discussed yet, right?}\cntodo{yes, I see the problem here. } 
%%%
%%%
%%% Results
The results of the experiments employing \textsc{DS} can be seen in Table \ref{tab:dagstuhl}. Generally, compared to the results on \texttt{AQCorpus}, the performance drops. This can be attributed to the domain-transfer. While \textsc{DS} also consist of web debate arguments, they consist of individual isolated arguments and not -- as our corpus -- of more complex texts. Training on our joint training set across all domains yields the highest correlation scores and generally, the annotations related to overall argument quality and reasonableness correlate best with our scores. To the best of our knowledge, we are the first to have a trained model in-place which is able to predict scores for fine-grained argument quality dimensions.

%\hfill
%\parbox{.49\linewidth}{
\begin{table}[th!]
\centering
\small
\begin{tabular}{llrrrrr}\toprule
\textbf{} &\textbf{} &\multicolumn{2}{c}{\textbf{Majority}} &\multicolumn{2}{c}{\textbf{Mean}} \\\cmidrule{3-6}
\textbf{Domain} &\textbf{Dimension} &\textbf{$r$} &\textbf{$\rho$} &\textbf{$r$} &\textbf{$\rho$} \\\midrule
All &Overall &\textbf{0.454} &\textbf{0.453} &\textbf{0.515} &\textbf{0.502} \\
&Cogency &0.382 &0.383 &0.443 &0.428 \\
&Effectiveness &0.406 &0.397 &0.478 &0.466 \\
&Reasonableness &0.427 &0.396 &0.492 &0.456 \\
\midrule
CQA forums &Overall &\textbf{0.425} &\textbf{0.424} &\textbf{0.475} &\textbf{0.473} \\
&Cogency &0.344 &0.343 &0.419 &0.407 \\
&Effectiveness &0.369 &0.369 &0.453 &0.454 \\
&Reasonableness &0.408 &0.393 &0.467 &0.447 \\
\midrule
Debate forums &Overall &0.365 &0.347 &0.423 &0.402 \\
&Cogency &0.306 &0.294 &0.364 &0.344 \\
&Effectiveness &0.338 &0.326 &0.419 &\textbf{0.404} \\
&Reasonableness &\textbf{0.398} &\textbf{0.355} &\textbf{0.431} &0.389 \\
\midrule
Review forums &Overall &0.315 &\textbf{0.312} &\textbf{0.346} &\textbf{0.335} \\
&Cogency &0.284 &0.276 &0.307 &0.302 \\
&Effectiveness &0.257 &0.260 &0.300 &0.303 \\
&Reasonableness &\textbf{0.325} &0.309 &0.338 &0.317 \\
\bottomrule
\end{tabular}
\caption{Pearson ($r$) and Spearman ($\rho)$ correlation coefficients when predicting with our \textsc{BERT MT$_{Flat}$} trained \emph{all-domain} or \emph{in-domain} on the Dagstuhl data. We correlate our prediction for each dimension with its associated true label when applying mean or majority aggregation on the annotations. Scores in bold indicate best performances per domain.}\label{tab:dagstuhl}
%}
\end{table}
